# Supplementary material for: Robust Finite-State Controllers for Uncertain POMDPs
Source: arXiv:2009.11459 source file (2021-03-04)
Supplement: Supplementary file 1 [file appendix.tex]

\section{Appendix}

In this appendix, we consider the dualization scheme for general POMDPs.
We first introduce the semi-infinite optimization problem for general POMDPs. 
Then introduce robust nonlinear programs, and highlight the differences in the dualization steps between a robust linear program (LP) and nonlinear program.
Finally, we define the dualization scheme for the semi-infinite constraints in the optimization problem for general POMDPs.

\section{Optimization Problem for uPOMDPs}

We now introduce the optimization problem with the nonnegative reward variables $\{r_s \geq 0\; | \; s \in S\}$ denoting the expected reward before reaching goal set $G$ from state s, and positive variables $\{\sched_{s,\act}> 0 \; | \; s \in S, \act \in \Act(s)\}$ denoting the probability of taking an action $\act$ in a state $s$ for the policy.
%Note that we only consider policies where for all states $s$ and actions $\alpha$ it holds that $\sched_{s,\act} > 0$, such that applying the policy to the uPOMDP does not change the underlying graph.%
\begin{flalign}
&\begin{aligned}
\text{maximize} \quad   & r_{s_I}
\end{aligned} \label{NLP:obj_g}\\
&\begin{aligned}
\text{subject to} \quad
% \end{aligned} \nonumber \\
%	&\begin{aligned}
\,\,  r_{s_I} \geq \kappa, \quad \forall s \in G, \quad & r_s = 0,
%    \end{aligned} \label{NLP:constraint:1}\\
%	&\begin{aligned}
%    \,\,    c_{s_I} \leq \kappa,
\end{aligned}  \label{NLP:constraint:2_g}\\
%&\begin{aligned} 
%
%    \end{aligned} \label{NLP:constraint:4}\\
%    &\begin{aligned} 
%    	\,\, & \forall s \in G. \quad & c_s = 0, 
%\end{aligned} \label{NLP:constraint:6}\\
&\begin{aligned} 
\forall s \in S, \quad  & \sum\nolimits_{\act \in \Act(s)} \sched_{s,\act} = 1,
\end{aligned} \label{NLP:constraint:3_g}\\
&\begin{aligned} 
\forall s, s' \in S \text{ s.t.\ } \ObsFun(s) = \ObsFun(s'), \forall \alpha \in \Act(s),\; \sigma_{s,\alpha} = \sched_{s',\alpha},
\end{aligned}\label{NLP:constraint:4_g}\\
&\begin{aligned} 
&\forall s \in S, \forall P \in \mathcal{P}, \;r_s \leq  \\
&\quad\sum_{\act \in \Act(s)}\sched_{s,\act}\cdot  \Big(\rew(s,\act) +  \sum_{s' \in S}  P(s,\act,s')\cdot r_{s'}\Big),
\end{aligned} \label{NLP:simple-nondet_g}\raisetag{0.7\baselineskip}
%    &\begin{aligned} &\forall s \in S \setminus G.\, \forall P \in \mathcal{P}. \\
%            & \,\, c_s \geq \sum_{\alpha \in Act} \sched_{s,\alpha} \cdot \Big( c(s,\alpha) + \sum_{s' \in S} P(s,\alpha,s') \cdot c_{s'} \Big)
%  \end{aligned} \label{NLP:constraint:7} \\
\end{flalign}%
where the objective and the constraints~\eqref{NLP:constraint:2_g}--\eqref{NLP:constraint:4_g} are as same as in the manuscript, and the constraint~\eqref{NLP:simple-nondet_g} encodes the computation of expected rewards for all states.

\begin{definition}[Robust nonlinear programs]
A robust nonlinear program (NLP) with the variables $x \in \R^n$ is 
\end{definition}
%We consider robust nonlinear programs\sj{Why is a robust LP a def, but this in flowtext?} in the form of\sj{You use $f$ above for soemthing else?}
%	\mc{rewrote here}
	%On the other hand\sj{which other hand}, if the functions in the constraints nonlinear in $x$\sj{are they nonlinear?},  such as 
	\begin{align}
		&\text{minimize} \quad c^\top x\\
	&\text{subject to} \quad \sum_{i=1}^n f_i(x)u_i + d^\top x \leq e \quad \forall u \in \mathcal{U}. \label{eq:robust_nonlinear}
	\end{align}
where $f_i, i=1,\ldots,n$ are nonlinear functions over $x$, $d \in \R^n,$ and $e \in \R$ are given data, $u\in \R^n$ is the uncertain parameter, and $\mathcal{U}$ is the uncertainty set.
	For such robust programs, we use a similar idea to reformulate the semi-infinite constraints with polytopic uncertainty set $\mathcal{U}$, that is defined by the linear inequalities $Cu+g\geq$ for $C \in \R^{m\times n}$. and $g \in \R^m$.
	 
	We write the Lagrangian of the maximization problem over  $\sum_{i=1}^m f_i(x)u_i$ with the dual variable $\mu\geq 0$ as
	\begin{align*}
	L(u,\mu) = \sum_{i=1}^n f_i(x)u_i + \mu^{\top}(Cu +g).
	\end{align*}

	Similar to the robust LPs, we take the supremum over $u$, and obtain
	\begin{align*}
	\underset{u \in \mathcal{U}}{\text{sup}} \;\;L(u,\mu)=   \begin{cases}
	\infty & \text{if } C_i^{\top}\mu + f_i \neq 0, \\
	\mu^\top g & \text{if } C_i^{\top}\mu + f_i = 0, i=1,\ldots,n
	\end{cases}
	\end{align*}
	where $C_i$ is the $i'$th row of the matrix $C$.
	Unlike robust LP's we do not have \emph{strong duality}.
	However, using \emph{weak duality}, we obtain 
	\begin{align*}
	\underset{u \in \mathcal{U}}{\text{sup}} \sum_{i=1}^m f_i(x)u_i \leq  \underset{\mu \geq 0}{\text{inf}} \lbrace \mu^\top f \;  |  \; C_i^{\top}\mu + &f_i(x) = 0, \\
	&\quad i=1,\ldots n \rbrace,
	\end{align*}
	where $C_i$ is the $i$'th row of the matrix $C$. 
	Note that, the left-hand side of the above equation is a \emph{lower bound} of the right-hand side, instead of being equal, a result of \emph{weak duality}.
	
	Therefore, for robust NLPs, we can obtain a conservative representation of the semi-infinite constraint~\eqref{eq:robust_nonlinear} with the following constraints
	\begin{align*}
	c^{\top}x+\mu^{\top}f \leq e, \;\; C_i^{\top}\mu + f_i(x) = 0, \;\; i=1,\ldots n, \quad \lambda \geq 0,
	\end{align*}
	which are finite. 
	Therefore, any feasible solution of $x$ to the above constraints is feasible to the constraint~\eqref{eq:robust_nonlinear}.

\subsection{Dualization for General uPOMDPs}

	We now describe the dualization of the semi-infinite constraints for general uPOMDPs. 
	The construction for general uPOMDPs will be similar to simple uPOMDPs. 
	However, unlike the case for simple uPOMDPs, the resulting finite set of constraints will no longer represent the semi-infinite constraints, and they will be a conservative reformulation.
	
	Similar to the manuscript, we assume that we have the matrices $C_{s,\act}$ and vectors $g_{s,\act}$ for each state $s \in S$ and action $\act \in \Act$ that describes the uncertain transition function.
	Then, we obtain a conservative reformulation of the constraints~\eqref{NLP:simple-nondet_g} as
	\begin{flalign}
	&\begin{aligned} 
	&\forall s \in S_{\mathrm{u}} \setminus T.\, 
	\,\, r_s \leq \sum_{\act \in \Act(s)} R(s,\act)\cdot \sched_{s',\act}+\mu^{\top}_{s,\act} g_{s,\act},\;\;\\
	&\forall \act \in \Act(s).\,\,\,
	C^\top_{s,\act}\mu_{s,\act}+q\cdot \sched_{s,\alpha}=0, \;\;\mu_{s,\act} \geq 0.\label{NLP:general-uncertain-finite}
	\end{aligned}
	\end{flalign}
	where $\mu_{s,\act}$ is the dual variable of the constraint $C_{s,\act}u+g_{s,\act}\geq 0$ and $q$ is an $|S|-$dimensional vector denoting the set of reward variables for each state $s \in S$. 
	
	We note that any feasible solution to the above constraints is also feasible to the constraints~\eqref{NLP:simple-nondet_g}.
	Therefore, the reformulation in~\eqref{NLP:general-uncertain-finite} preserves the soundness of the optimization problem.
	We also note that the above constraints are \emph{quadratic} as the probability variables in $\vec{p}_{s,\act}$ are multiplied with the policy variables $\sched_{s,\alpha}$.
	However, the set of constraints is finite. 
	Therefore the resulting optimization problem is a finite-dimensional nonconvex problem.
